# Supplementary material for: Pushing the performances of ASR models on English and Spanish accents
Source: arXiv:2212.12048 source file (2022-12-22)
Supplement: Supplementary file 1 [file arch_cpcw2v.tex]

\begin{table}[h!]
    \centering
    \begin{tabular}{c|c}
    \toprule
      Layer  & Output Shape \\
      \midrule
        MFSC &  \\
        Layer Norm (axis 0 1 2) & \\
        Conv1D W 2 S 1 P -1 & \\
        GatedLinearUnit & \\
        Dropout 0.05 + Reshape \\
        SINPOSEMB & \\
        
    \bottomrule
    \end{tabular}
    \caption{
      \textbf{WER MTL Loss}
    \label{tab:mtl}}
\end{table}
