# Supplementary material for: Pushing the performances of ASR models on English and Spanish accents
Source: arXiv:2212.12048 source file (2022-12-22)
Supplement: Supplementary file 3 [file combo_emformer_es_backup.tex]

\begin{table*}[h!]
    \centering
    \begin{tabular}{c|cc|c}
    \toprule
      accent & Emformer baseline & W/ accent classifier,pretrained encoder & \% change\\
      \midrule
      es\_ar & 14.36 & 13.38 & -6.80\%\\
      es\_es & 13.03 & 11.92 & -8.52\%\\
      es\_gt & 13.55 & 12.58 & -7.20\%\\
      es\_pe & 15.15 & 14.16 & -6.52\%\\
      es\_ve & 15.57 & 14.53 & -6.64\%\\
      es\_latam & 13.52 & 12.40 & -8.31\%\\
    \midrule
      average & 14.19 & 13.16 & -7.29\%\\
    \bottomrule
    \end{tabular}
    \caption{
      \textbf{WER with auxiliary accent prediction task on Emformer model with pretrained encoder weightsfor Spanish}
    \label{tab:accentPlusPretrain}}
\end{table*}
