# Supplementary material for: Pushing the performances of ASR models on English and Spanish accents
Source: arXiv:2212.12048 source file (2022-12-22)
Supplement: Supplementary file 4 [file mtl_emformer_es_backup.tex]

\begin{table*}[h!]
    \centering
    \begin{tabular}{c|ccccccc|c}
    \toprule
      aux accent classifier & es\_ar & es\_es & es\_gt & es\_pe & es\_ve & es\_latam & avg wer & \% change\\
      \midrule
      without accent prediction (baseline) & 14.36 & 13.03 & 13.55 & 15.15 & 15.57 & 13.52 & 14.19 & -\\
      all, low, $\lambda_{aux\_accent} 0.1$, $\lambda_{aux\_asr} 0.9$ & 14.14 & 12.59 & 13.32 & 14.91 & 15.39 & 13.27 & 13.94 & -1.76\%\\
      clean, low, $\lambda_{aux\_accent} 0.1$, $\lambda_{aux\_asr} 0.9$ & 14.05 & 12.74 & 13.30 & 14.84 & 15.40 & 13.24 & 13.93 & -1.83\%\\
      clean, low, $\lambda_{aux\_accent} 0.2$, $\lambda_{aux\_asr} 0.8$ & 14.17 & 12.76 & 13.35 & 14.88 & 15.45 & 13.39 & 14.00 & -1.34\%\\
      clean, mid, $\lambda_{aux\_accent} 0.1$, $\lambda_{aux\_asr} 0.9$ & 13.98 & 12.54 & 13.34 & 14.88 & 15.41 & 13.27 & 13.90 & \textbf{-2.40\%}\\
      clean, mid, $\lambda_{aux\_accent} 0.2$, $\lambda_{aux\_asr} 0.8$ & 14.08 & 12.80 & 13.37 & 14.99 & 15.40 & 13.36 & 14.00 & -1.34\% \\
      all, top, $\lambda_{aux\_accent} 0.1$, $\lambda_{aux\_asr} 0.9$ & 14.11 & 12.57 & 13.32 & 14.98 & 15.38 & 13.39 & 13.96 & -1.62\%\\\
      clean, top, $\lambda_{aux\_accent} 0.1$, $\lambda_{aux\_asr} 0.9$ & 14.04 & 12.56 & 13.30 & 15.00 & 15.42 & 13.28 & 13.93 & -1.83\%\\\

    \bottomrule
    \end{tabular}
    \caption{
      \textbf{WER with auxiliary accent prediction task on Emformer model for Spanish}
    \label{tab:mtlUsageSpanish}}
\end{table*}\begin{table*}[h!]
    \centering
    \begin{tabular}{c|cc|c}
    \toprule
      accent & Emformer baseline & W/ accent classifier,pretrained encoder & \% change\\
      \midrule
      es\_ar & 14.36 & 13.38 & -6.80\%\\
      es\_es & 13.03 & 11.92 & -8.52\%\\
      es\_gt & 13.55 & 12.58 & -7.20\%\\
      es\_pe & 15.15 & 14.16 & -6.52\%\\
      es\_ve & 15.57 & 14.53 & -6.64\%\\
      es\_latam & 13.52 & 12.40 & -8.31\%\\
    \midrule
      average & 14.19 & 13.16 & -7.29\%\\
    \bottomrule
    \end{tabular}
    \caption{
      \textbf{WER with auxiliary accent prediction task on Emformer model with pretrained encoder weightsfor Spanish}
    \label{tab:accentPlusPretrain}}
\end{table*}\begin{table*}[h!]
    \centering
    \begin{tabular}{c|cc|c}
    \toprule
      accent & Emformer baseline & W/ accent classifier,pretrained encoder & \% change\\
      \midrule
      es\_ar & 14.36 & 13.38 & -6.80\%\\
      es\_es & 13.03 & 11.92 & -8.52\%\\
      es\_gt & 13.55 & 12.58 & -7.20\%\\
      es\_pe & 15.15 & 14.16 & -6.52\%\\
      es\_ve & 15.57 & 14.53 & -6.64\%\\
      es\_latam & 13.52 & 12.40 & -8.31\%\\
    \midrule
      average & 14.19 & 13.16 & -7.29\%\\
    \bottomrule
    \end{tabular}
    \caption{
      \textbf{WER with auxiliary accent prediction task on Emformer model with pretrained encoder weightsfor Spanish}
    \label{tab:accentPlusPretrain}}
\end{table*}
