# Supplementary material for: Pushing the performances of ASR models on English and Spanish accents
Source: arXiv:2212.12048 source file (2022-12-22)
Supplement: Supplementary file 5 [file mtl_enformer_en_backup.tex]

\begin{table}[h!]
    \centering
    \begin{tabular}{c|c|c}
    \toprule
      aux accent classifier & avg wer & \% change\\
      \midrule
      without accent prediction (baseline) & 14.19 & -\\
      low, $1.0$, $\lambda_{aux\_asr} 1.0$ & 20.58 & +3.46\%\\
      mid, $\lambdaacc1.0$, $\lambda_{aux\_asr} 1.0$ & 20.59 & +3.57\%\\
      top, $\lambdaacc1.0$, $\lambda_{aux\_asr} 1.0$ & 21.36 & +7.41\%\\
      low, $\lambdaacc0.5$, $\lambda_{aux\_asr} 1.0$ & 20.23 & +1.71\%\\
      mid, $\lambdaacc0.5$, $\lambda_{aux\_asr} 1.0$ & 20.11 & +1.11\%\\
      top, $\lambdaacc0.5$, $\lambda_{aux\_asr} 1.0$ & 20.57 & +3.43\%\\
      low, $\lambdaacc0.1$, $\lambda_{aux\_asr} 0.9$ & 19.67 & -1.08\%\\
      mid, $\lambdaacc0.1$, $\lambda_{aux\_asr} 0.9$ & 19.59 & \textbf{-1.52\%}\\
      top, $\lambdaacc0.1$, $\lambda_{aux\_asr} 0.9$ & 19.74 & -1.04\%\\
    \bottomrule
    \end{tabular}
    \caption{
      \textbf{WER with auxiliary accent prediction task on Emformer model for English}
    \label{tab:mtlUsageEnglishAll}}
\end{table}
